# Supplementary material for: Through Iron & Ice: Searching for Sterile Neutrinos at the IceCube Neutrino Observatory
Source: arXiv:2210.09418 source file (2022-10-17)
Supplement: Supplementary file 1 [file prd_supp2.pdf]

# Supplemetary Material: Significant Excess of Electron-Like Events in the MiniBooNE Short-Baseline Neutrino Experiment

A. A. Aguilar-Arevalo[13], B. C. Brown[6], L. Bugel[12], G. Cheng[5], J. M. Conrad[12], R. L. Cooper[10,15], R. Dharmapalan[1,2], A. Diaz[12], Z. Djurcic[2], D. A. Finley[6], R. Ford[6], F. G. Garcia[6], G. T. Garvey[10], J. Grange[7], E.-C. Huang[10], W. Huelsnitz[10], C. Ignarra[12], R. A. Johnson[3], G. Karagiorgi[5], T. Katori[12,16], T. Kobilarcik[6], W. C. Louis[10], C. Mariani[19], W. Marsh[6], G. B. Mills[10,†], J. Mirabal[10], J. Monroe[18], C. D. Moore[6], J. Mousseau[14], P. Nienaber[17], J. Nowak[9], B. Osmanov[7], Z. Pavlovic[6], D. Perevalov[6], H. Ray[7], B. P. Roe[14], A. D. Russell[6], M. H. Shaevitz[5], J. Spitz[14], I. Stancu[1], R. Tayloe[8], R. T. Thornton[10], M. Tzanov[4,11], R. G. Van de Water[10], D. H. White[10], D. A. Wickremasinghe[3], E. D. Zimmerman[4]

(The MiniBooNE Collaboration)

[1]*University of Alabama; Tuscaloosa, AL 35487, USA*
[2]*Argonne National Laboratory; Argonne, IL 60439, USA*
[3]*University of Cincinnati; Cincinnati, OH, 45221, USA*
[4]*University of Colorado; Boulder, CO 80309, USA*
[5]*Columbia University; New York, NY 10027, USA*
[6]*Fermi National Accelerator Laboratory; Batavia, IL 60510, USA*
[7]*University of Florida; Gainesville, FL 32611, USA*
[8]*Indiana University; Bloomington, IN 47405, USA*
[9]*Lancaster University; Lancaster LA1 4YB, UK*
[10]*Los Alamos National Laboratory; Los Alamos, NM 87545, USA*
[11]*Louisiana State University; Baton Rouge, LA 70803, USA*
[12]*Massachusetts Institute of Technology; Cambridge, MA 02139, USA*
[13]*Instituto de Ciencias Nucleares; Universidad Nacional Autónoma de México; CDMX 04510, México*
[14]*University of Michigan; Ann Arbor, MI 48109, USA*
[15]*New Mexico State University; Las Cruces, NM 88003, USA*
[16]*Queen Mary University of London; London E1 4NS, UK*
[17]*Saint Mary's University of Minnesota; Winona, MN 55987, USA*
[18]*Royal Holloway, University of London; Egham TW20 0EX, UK*
[19]*Center for Neutrino Physics; Virginia Tech; Blacksburg, VA 24061, USA*
[†]*Deceased*

(Dated: September 26, 2018)

## Appendix: Background Determination & Data vs Monte Carlo Comparisons

Almost all of the backgrounds in the electron-neutrino candidate event sample are determined directly from MiniBooNE data [26]. The muon-neutrino charged-current quasi-elastic (CCQE) observed data sample allows the background determination of both mis-identified $\nu_\mu$ CCQE events from pion decay [28] and $\nu_e$ CCQE events from muon decay, as the neutrinos come from the same parent pion and $\nu_e$ and $\nu_\mu$ cross sections are the same from lepton universality after correcting for charged lepton mass effects. The $\nu_e$ CCQE background from kaon decay was determined from external measurements and confirmed by data from the SciBooNE experiment [27]. In addition, the neutral current (NC) $\pi^0$ data sample allows the background determination of both NC $\pi^0$ events [32] and single gamma events from $\Delta \rightarrow N\gamma$ decays. Various theoretical estimates [30, 31] have confirmed the MiniBooNE single gamma background estimate. Fig. 1 shows a comparison of the single gamma background estimate from reference [31] with that of MiniBooNE, where good agreement is obtained. Single-gamma backgrounds from external neutrino interactions ("dirt" backgrounds) are estimated using topological and spatial cuts to isolate the events whose vertices are near the edge of the detector and point towards the detector center [34]. These estimates have been confirmed by preliminary measurements of the absolute event time reconstruction of electron-neutrino candidate events, where a fit to the dirt event background using timing agrees within 10% with the background estimate using topological and spatial cuts.

In order to demonstrate that the MiniBooNE background estimates are reliable, various comparisons between the neutrino data, corresponding to $12.84 \times 10^{20}$ protons on target (POT), and the Monte Carlo simulation have been performed to check and confirm the accuracy of the simulation. Fig. 2 shows an absolute comparison of the $\pi^0$ reconstructed mass distribution between the data and the simulation for NC $\pi^0$ events. Excellent agreement is obtained, and the ratio of the number of data events (42,483) to the number of Monte Carlo events (42,530) in the mass range from 80 to 200 MeV/c$^2$ is equal to 0.999. Fig. 3 shows an absolute comparison of

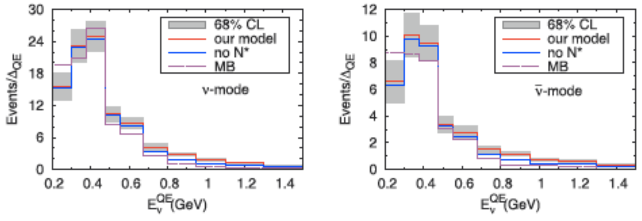


FIG. 1: A comparison of the single gamma background estimate from reference [31] with that of MiniBooNE, where good agreement is obtained.

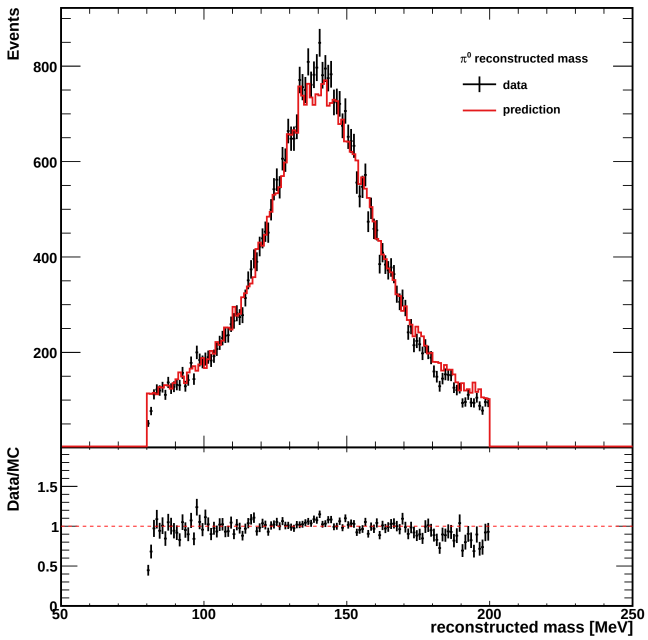


FIG. 2: An absolute comparison of the $\pi^0$ reconstructed mass distribution between the neutrino data ($12.84 \times 10^{20}$ POT) and the simulation for NC $\pi^0$ events (top). Also shown is the ratio between the data and Monte Carlo simulation (bottom). The error bars show only statistical uncertainties.

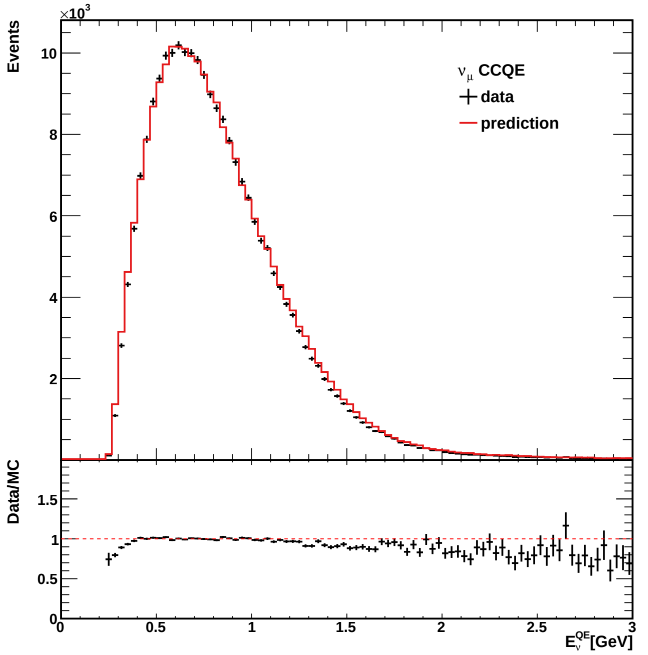


FIG. 3: An absolute comparison of the reconstructed neutrino energy distribution for CCQE events between the neutrino data ($12.84\times10^{20}$ POT) and the simulation (top). Also shown is the ratio between the data and Monte Carlo simulation (bottom). The error bars show only statistical uncertainties.

the reconstructed neutrino energy distribution for CCQE events between the data and the simulation. Excellent agreement is also obtained, and the ratio of the number of data events (232,096) to the number of Monte Carlo events (236,145) is equal to 0.983.

In order to check the particle identification (PID) cuts, Figs. 4, 5, and 6 show comparisons between the data and simulation for the electron-muon likelihood distribution, the electron-pion likelihood distribution, and the gamma-gamma mass distribution. In each figure, distributions are shown after successive cuts are applied: no PID cut, electron-muon likelihood cut, electron-muon plus electron-pion likelihood cuts, and electron-muon plus electron-pion likelihood cuts and a gamma-gamma mass cut. The last plot in each figure shows distributions with the final event selection. The vertical lines in the figures show the range of energy-dependent cut values. Good agreement between the data and the simulation is obtained outside the cut values, while an excess of events is observed inside the cut values. Figs. 7 and 8 show the momentum and gamma-gamma opening angle distributions after successive cuts are applied. Good agreement is obtained between the data and Monte Carlo simulation for the no PID cut distributions, while event excesses are observed after the final event selection. These five plots also demonstrate that sidebands show good agreement between the data and simulation.

Fig. 9 shows the visible energy (Evis) and $\cos\theta_e$ (Uz) distributions for the electron-neutrino candidate events in neutrino mode (top) and antineutrino mode (bottom). Also shown in the figures are the expectations from all known backgrounds and from the oscillation best fit. These distributions are important because the reconstructed neutrino energy, $E_\nu^{QE}$, is determined from Evis and Uz. A check on the spatial reconstruction is shown

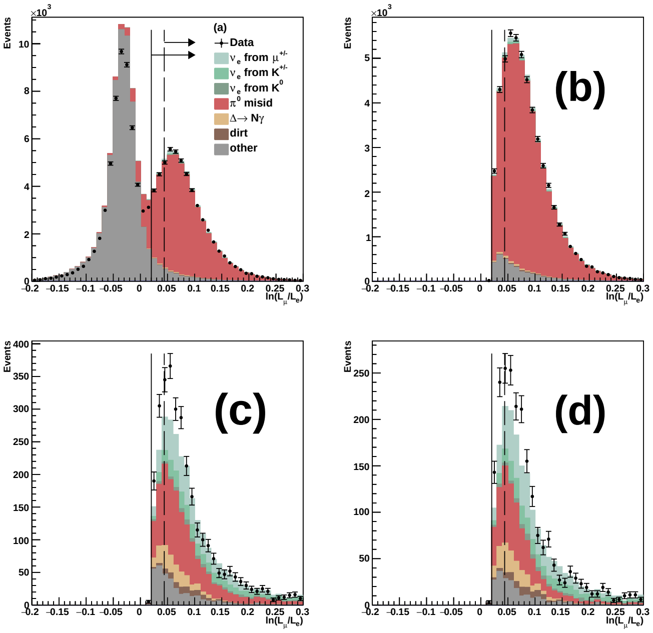


FIG. 4: Comparisons between the data and simulation for the electron-muon likelihood distribution after successive cuts are applied: (a) no PID cut, (b) electron-muon likelihood cut, (c) electron-muon plus electron-pion likelihood cuts, and (d) electron-muon plus electron pion likelihood cuts plus a gamma-gamma mass cut. The vertical lines in the figures show the range of energy-dependent cut values. The error bars show only statistical uncertainties.

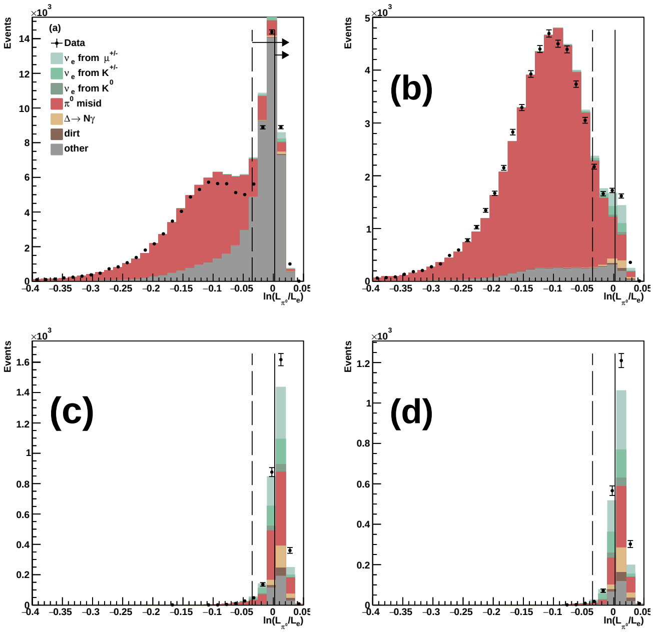


FIG. 5: Comparisons between the data and simulation for the electron-pion likelihood distribution after successive cuts are applied: (a) no PID cut, (b) electron-muon likelihood cut, (c) electron-muon plus electron-pion likelihood cuts, and (d) electron-muon plus electron pion likelihood cuts plus a gamma-gamma mass cut. The vertical lines in the figures show the range of energy-dependent cut values. The error bars show only statistical uncertainties.

in Fig. 10, where the radius reconstruction in the data is compared to the Monte Carlo simulation. As shown in the figure, the event excess is evenly distributed up to the 5m radius cut. A further check of the electron efficiency was obtained from the reconstruction of electron events in MiniBooNE that originated from the off-axis NUMI beam (P. Adamson et al., Phys. Rev. Lett. **102**, 211801 (2009)), as the intrinsic $\nu_e$ background was approximately ten times higher in the NUMI beam than in the BNB. The measured electron rate agreed with the simulation within errors.

### Appendix: Stability Checks

Many checks have been performed on the data, including beam and detector stability checks. Fig. 11 shows the total number of neutrino events observed per $10^{17}$ POT over the lifetime of MiniBooNE in neutrino mode, antineutrino mode and beam-dump mode. The neutrino mode event rate of 100 events per $10^{17}$ POT has been stable to $< 2\%$ over the 15 year MiniBooNE running period. This is within the expected errors from time variations in BNB performance, such as target/horn change, beam rate monitoring, etc. A small change in the detector energy response between the first and second neutrino data set has been corrected by increasing the measured energy in the second data set by 2%. About half of the energy change is from PMT failures in the intervening years, and the remainder is within the detector response error from gain variations, oil properties, etc. With this energy correction, the first and second data sets are found to agree well. Fig. 12 compares the reconstructed $\nu_\mu$ CCQE energy distributions for the second data set in 2016 and 2017 to the first data set, where good agreement is obtained. Likewise, Fig. 13 shows that the $\pi^0$ mass distribution has also not changed.

### Appendix: Comparing New and Old Neutrino Data

Figs. 14 and 15 show the $E_\nu^{QE}$ distribution for $\nu_e$ CCQE data and background in neutrino mode over the full available energy range for the first $6.46 \times 10^{20}$ POT data set and the second $6.38 \times 10^{20}$ POT data set. Fig. 16 shows the $\nu_e$ CCQE data and background in antineutrino mode. Each bin of reconstructed $E_\nu^{QE}$ corresponds to a distribution of "true" generated neutrino energies, which can overlap adjacent bins. Note that the 162.0 event excess in the $6.46 \times 10^{20}$ POT data is approximately $1\sigma$ lower than the average excess, while the 219.2 event excess in the $6.38 \times 10^{20}$ POT data is approximately $1\sigma$ higher than the average excess. In antineutrino mode, a total of 478 data events pass the $\nu_e$ CCQE event selection requirements with $200 < E_\nu^{QE} <$ 1250 MeV, compared to a background expectation of

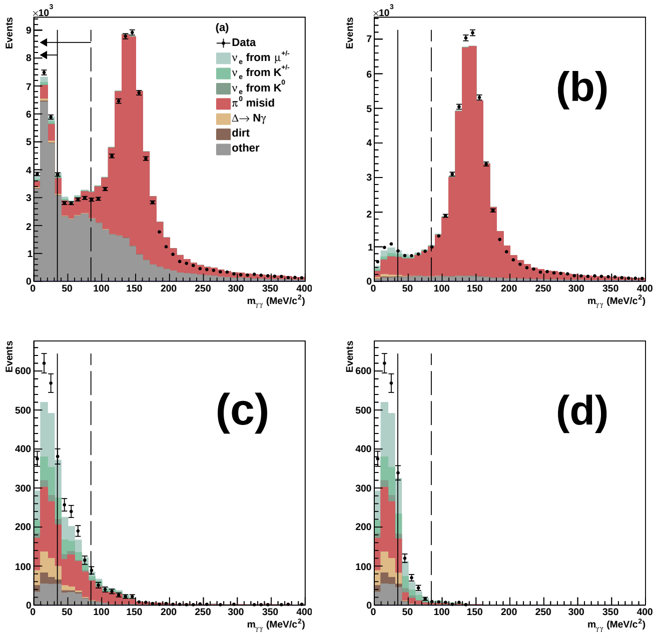


FIG. 6: Comparisons between the data and simulation for the gamma-gamma mass distribution after successive cuts are applied: (a) no PID cut, (b) electron-muon likelihood cut, (c) electron-muon plus electron-pion likelihood cuts, and (d) electron-muon plus electron pion likelihood cuts plus a gamma-gamma mass cut. The vertical lines in the figures show the range of energy-dependent cut values. The error bars show only statistical uncertainties.

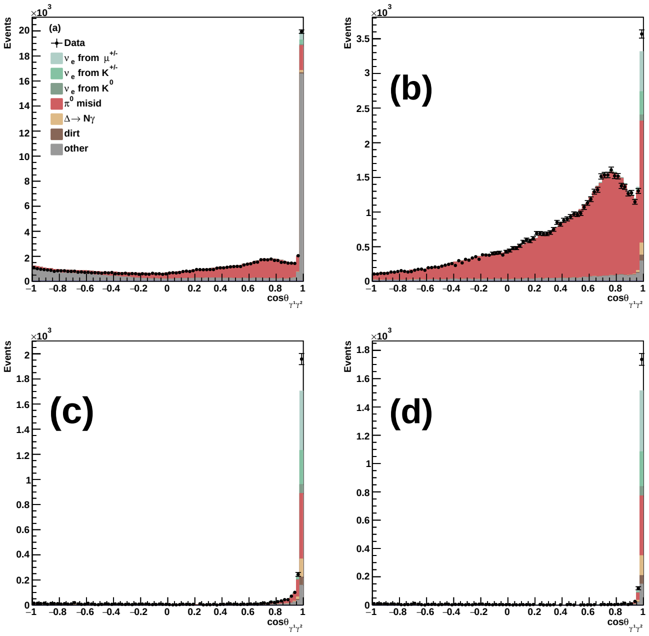


FIG. 8: Comparisons between the data and simulation for the gamma-gamma opening angle distribution after successive cuts are applied: (a) no PID cut, (b) electron-muon likelihood cut, (c) electron-muon plus electron-pion likelihood cuts, and (d) electron-muon plus electron pion likelihood cuts plus a gamma-gamma mass cut. The event excess occurs almost entirely for opening angles less than 13 degrees. The error bars show only statistical uncertainties.

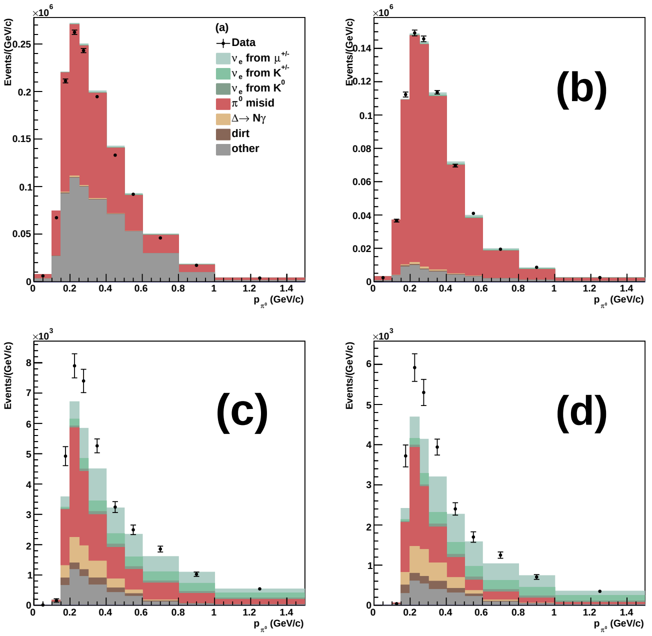


FIG. 7: Comparisons between the data and simulation for the momentum distribution after successive cuts are applied: (a) no PID cut, (b) electron-muon likelihood cut, (c) electron-muon plus electron-pion likelihood cuts, and (d) electron-muon plus electron pion likelihood cuts plus a gamma-gamma mass cut. The error bars show only statistical uncertainties.

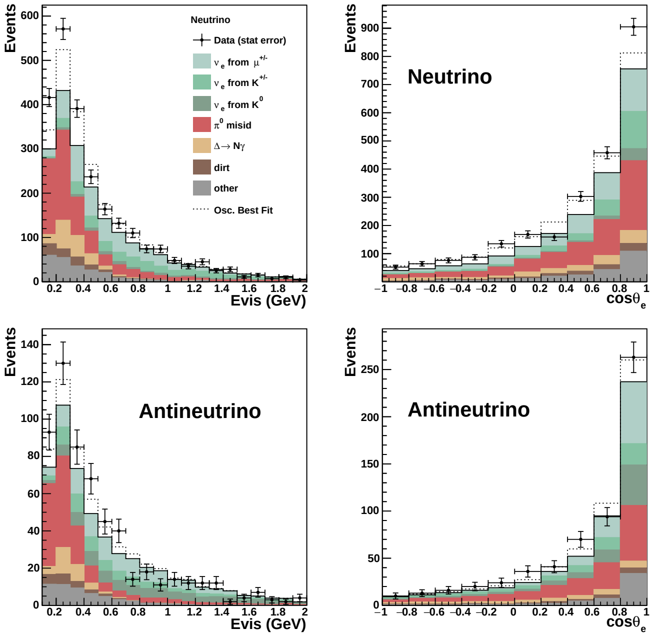


FIG. 9: The visible energy (Evis) and $\cos\theta_e$ (Uz) distributions for the electron-neutrino candidate events in neutrino mode (top) and antineutrino mode (bottom). (The error bars show only statistical uncertainties.) Also shown in the figure are the expectations from all known backgrounds and from the oscillation best fit.

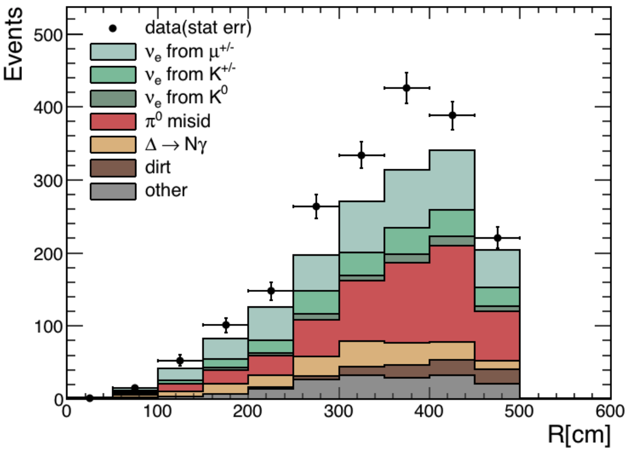


FIG. 10: The radius reconstruction in the data is compared to the Monte Carlo simulation. The event excess is evenly distributed up to the 5m radius cut.

$398.7 \pm 20.0(stat.) \pm 20.5(syst.)$ events. The excess is then $79.3 \pm 28.6$ events or a $2.8\sigma$ effect.

---


[1] C. Athanassopoulos *et al.*, Phys. Rev. Lett. 75, 2650 (1995); 77, 3082 (1996); 81, 1774 (1998); Phys. Rev. C. **54**, 2685 (1996); **58**, 2489 (1998); A. Aguilar *et al.*, Phys. Rev. D 64, 112007 (2001).

[2] A. A. Aguilar-Arevalo *et al.*, Phys. Rev. Lett. 98, 231801 (2007); Phys. Rev. Lett. 102, 101802 (2009); Phys. Rev. Lett. 105, 181801 (2010).

[3] A. A. Aguilar-Arevalo *et al.*, Phys. Rev. Lett. 110, 161801 (2013).

[4] G. Mention, M. Fechner, T. Lasserre, T. A. Mueller, D. Lhuillier, M. Cribier, and A. Letourneau, Phys. Rev. D 83, 073006 (2011).

[5] C. Giunti and M. Laveder, Phys. Rev. C 83, 065504 (2011).

[6] M. Sorel, J. M. Conrad and M. H. Shaevitz, Phys. Rev. D 70, 073004 (2004).

[7] G. Karagiorgi, Z. Djurcic, J. M. Conrad, M. H. Shaevitz and M. Sorel, Phys. Rev. D 80, 073001 (2009); D 81, 039902(E) (2010).

[8] G.H. Collin, C.A. Argüelles, J.M. Conrad, and M.H. Shaevitz, Phys. Rev. Lett. 117, 221801 (2016).

[9] C. Giunti and M. Laveder, Phys. Lett. B 706, 200 (2011); Phys. Rev. D84, 073008, (2011).

[10] S. Gariazzo, C. Giunti, M. Laveder, and Y.F. Li, arXiv:1703.00860 [hep-ph] (2017).

[11] J. Kopp, M. Maltoni and T. Schwetz, Phys. Rev. Lett. 107, 091801 (2011); Joachim Kopp, Pedro A.N. Machado, Michele Maltoni, and Thomas Schwetz, JHEP 1305, 050, (2013).

[12] Mona Dentler, Alvaro Hernandez-Cabezudo, Joachim Kopp, Pedro Machado, Michele Maltoni, Ivan Martinez-Soler, and Thomas Schwetz, arXiv:1803.10661 [hep-ph] (2018).

[13] K. N. Abazajian et al., arXiv:1204.5379 [hep-ph] (2012).

[14] J. M. Conrad, C. M. Ignarra, G. Karagiorgi, M. H. Shaevitz, and J. Spitz, arXiv:1207.4765 [hep-ex] (2012).

[15] J. Asaadi, E. Church, R. Guenette, B. J. P. Jones, and A. M. Szelc, Phys. Rev. D 97, 075021 (2018); G. Karagiorgi, M. H. Shaevitz, and J. M. Conrad, arXiv:1202.1024; Heinrich Paes, Sandip Pakvasa, and Thomas J. Weiler, Phys. Rev. D 72, 095017 (2005); Dominik Doring, Heinrich Paes, Philipp Sicking, and Thomas J. Weiler, arXiv:1808.07460 [hep-ph] (2018).

[16] V. A. Kostelecky and M. Mewes, Phys. Rev. D 69, 016005 (2004); T. Katori, V. A. Kostelecky, and R. Tayloe, Phys. Rev. D 74, 105009 (2006); Jorge S. Diaz and V. A. Kostelecky, Phys. Lett. B 700, 25 (2011); Jorge S. Diaz and V. A. Kostelecky, Phys. Rev. D 85, 016013 (2012).

[17] S. N. Gninenko, Phys. Rev. Lett. 103, 241802 (2009); S. N. Gninenko and D. S. Gorbunov, Phys. Rev. D 81, 075013 (2010); Yang Bai, Ran Lu, Sida Lu, Jordi Salvado, and Ben A. Stefanek, Phys. Rev. D 93, 073004 (2016); Zander Moss, Marjon H. Moulai, Carlos Argüelles, Janet M. Conrad, Phys. Rev. D 97, 055017 (2018); Enrico Baertuzzo, Sudip Jana, Pedro A. N. Machado, and Renata Zukanovich Funchal, arXiv:1807.09877 [hep-ph] (2018); Peter Ballett, Silvia Pascoli, and Mark Ross-Lonergan, arXiv:1808.02915 [hep-ph] (2018).

[18] Jiajun Liao and Danny Marfatia, Phys. Rev. Lett. 117, 071802 (2016).

[19] Marcela Carena, Ying-Ying Li, Camila S. Machado, Pedro A. N. Machado, Carlos E. M. Wagner, Phys. Rev. D 96, 095014 (2017).

[20] A. A. Aguilar-Arevalo *et al.*, Phys. Rev. D 79, 072002 (2009).

[21] A. A. Aguilar-Arevalo *et al.*, Nucl. Instrum. Meth. A 599, 28 (2009).

[22] R. B. Patterson *et al.*, Nucl. Instrum. Meth. A 608, 206 (2009).

[23] A. A. Aguilar-Arevalo *et al.*, Phys. Rev. D 81, 092005 (2010); A. A. Aguilar-Arevalo *et al.*, Phys. Rev. D 88, 032001 (2013).

[24] A. A. Aguilar-Arevalo *et al.* [MiniBooNE Collaboration], Phys. Rev. Lett. **118**, no. 22, 221803 (2017); arXiv:1807.06137.

[25] A. A. Aguilar-Arevalo *et al.*, Phys. Rev. D 84, 072005 (2011).

[26] R. B. Patterson, Ph.D. Thesis, Princeton University (2007), http://www-boone.fnal.gov/publications/Papers/rbpatter_thesis.pdf.

[27] G. Cheng *et al.*, Phys. Rev. D 84, 012009 (2011); C. Mariani, G. Cheng, J. M. Conrad and M. H. Shaevitz, Phys. Rev. D **84**, 114021 (2011).

[28] A. A. Aguilar-Arevalo *et al.*, Phys. Rev. D 81, 092005 (2010); Phys. Rev. Lett. 100, 032301 (2008).

[29] A. A. Aguilar-Arevalo *et al.*, Phys. Rev. D 83, 052007 (2011); Phys. Rev. Lett. 103, 081801 (2009).

[30] V. P. Efrosinin, Yu. G. Kudenko, and A. N. Khotjantsev, Phys. Atom. Nucl. 72, 459 (2009); Richard J. Hill, Phys. Rev. D 81, 013008 (2010); Richard J. Hill, Phys. Rev. D 84, 017501 (2011); Xilin Zhang and Brian D. Serot, Phys. Lett. B719, 409 (2013); Phys. Rev. C **86**, 035502 (2012); Phys. Rev. C **86**, 035504 (2012); Brian D. Serot and Xilin Zhang, Phys. Rev. C **86**, 015501 (2012).

[31] E. Wang, L. Alvarez-Ruso, and J. Nieves, Phys. Rev. C **89**, 015503 (2014); Phys. Lett. B740, 16 (2015).

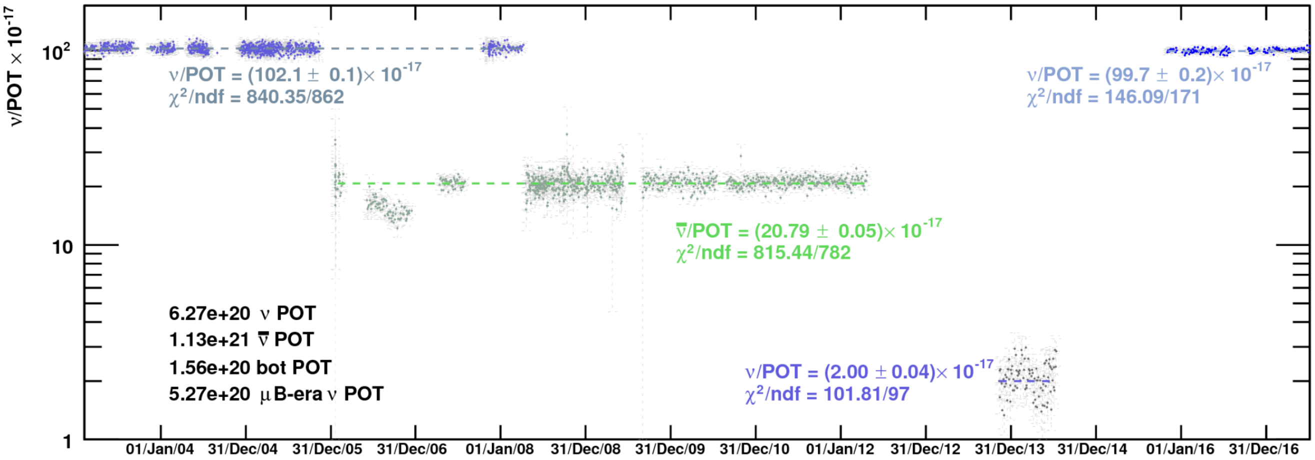


FIG. 11: The total number of neutrino events observed per $10^{17}$ POT over the lifetime of MiniBooNE in neutrino mode, antineutrino mode and beam-dump mode.


[32] A. A. Aguilar-Arevalo *et al.*, Phys. Rev. D 81, 013005 (2010); Phys. Lett. B. 664, 41 (2008).

[33] D. Rein and L. M. Sehgal, Phys. Lett. B. 104, 394 (1981); S. S. Gershtein, Yu. Ya. Komachenko, and M. Yu. Khlopov, Sov. J. Nucl. Phys. 33, 860 (1981); Jeffrey A. Harvey, Christopher T. Hill, and Richard J. Hill, Phys. Rev. Lett. 99, 261601 (2007); J. P. Jenkins and T. Goldman, Phys. Rev. D 80, 053005 (2009); Artur M. Ankowski, Omar Benhar, Takaaki Mori, Ryuta Yamaguchi, and Makoto Sakuda, Phys. Rev. Lett. 108, 052505 (2012); K. M. Graczyk, D. Kielczewska, P. Przewlocki, J. T. Sobczyk, Phys. Rev. D 80, 093001 (2009).

[34] A. A. Aguilar-Arevalo *et al.*, Phys. Rev. Lett. 102, 101802 (2009).

[35] M. Martini, M. Ericson, G. Chanfray, and J. Marteau, Phys. Rev. C **80**, 065501 (2009); M. Martini, M. Ericson, and G. Chanfray, Phys. Rev. D **85**, 093012 (2012); Phys. Rev. D **87**, 013009 (2013); D. Meloni and M. Martini, Phys. Lett. B. 716, 186 (2012); J. Nieves, I. R. Simo, and M. J. Vicente Vacas, Phys. Rev. C 83, 045501 (2011); J. Nieves, F. Sanchez, I. R. Simo, and M. J. Vicente Vacas, Phys. Rev. D 85, 113008 (2012); O. Lalakulich, K. Gallmeister, and U. Mosel, Phys. Rev. C **86**, 014614 (2012); Ulrich Mosel, Olga Lalakulich, and Kai Gallmeister, Phys. Rev. Lett. 112, 151802 (2014); Andrea Meucci and Carlotta Giusti, Phys. Rev. D 85, 093002 (2012); G. D. Megias *et al.*, Phys. Rev. D 91, 073004 (2015); P. Coloma and P. Huber, Phys. Rev. Lett. 111, 221802 (2013); Jan. T. Sobczyk, Phys. Rev. C 86, 015504 (2012).

[36] M. Ericson, M. V. Garzelli, C. Giunti, and M. Martini, Phys. Rev. D 93, 073008 (2016).

[37] B. Armbruster *et al.*, Phys. Rev. D 65, 112001 (2002).

[38] N. Agafonova *et al.*, arXiv1803.11400 [hep-ex] (2018).

[39] M. Antonello *et al.*, arXiv:1503.01520 (2015).

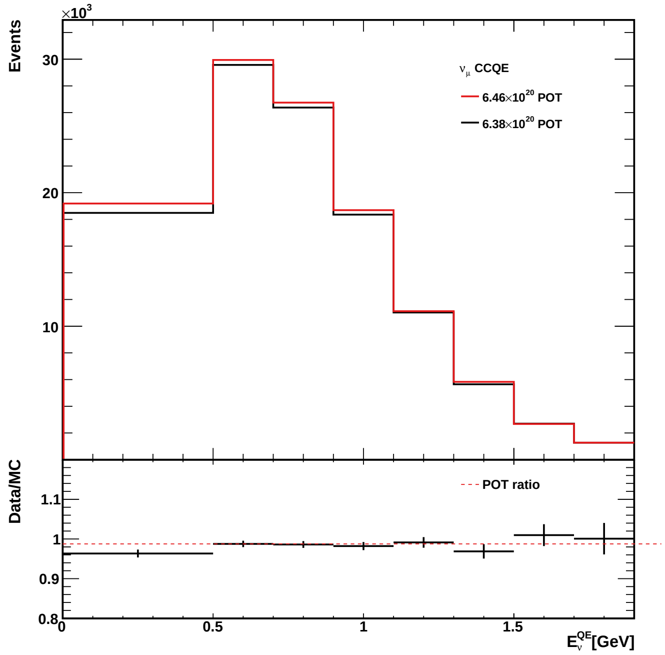


FIG. 12: The top plot shows a comparison between the reconstructed $\nu_\mu$ CCQE energy distributions for the second data set in 2016 and 2017 ($6.38 \times 10^{20}$ POT) to the first data set ($6.46 \times 10^{20}$ POT). The bottom plot shows the ratio of the second data set to the first data set.

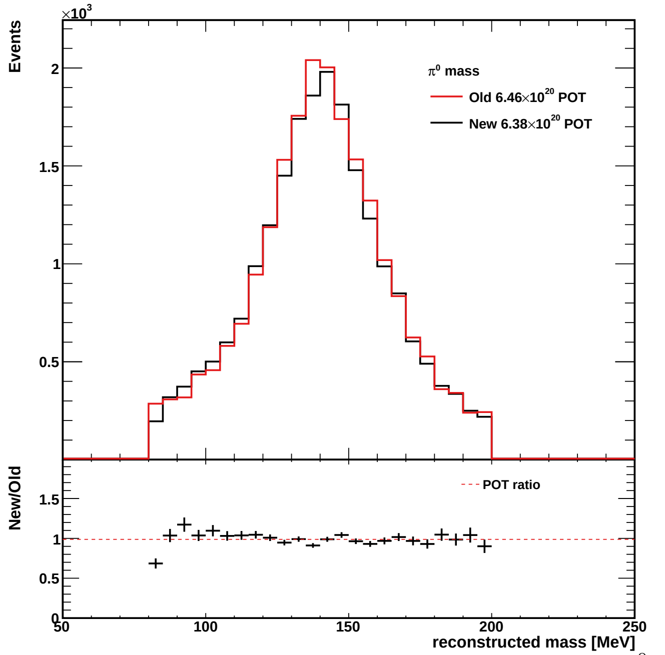


FIG. 13: The top plot shows a comparison between the $\pi^0$ mass distributions for the second data set in 2016 and 2017 ($6.38 \times 10^{20}$ POT) to the first data set ($6.46 \times 10^{20}$ POT). The bottom plot shows the ratio of the second data set to the first data set.

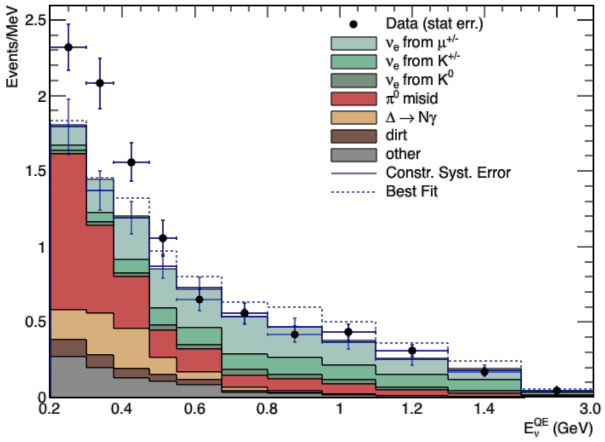


FIG. 14: The neutrino mode $E_\nu^{QE}$ distributions, corresponding to the first $6.46 \times 10^{20}$ POT data set, for $\nu_e$ CCQE data (points with statistical errors) and background (histogram with systematic errors).

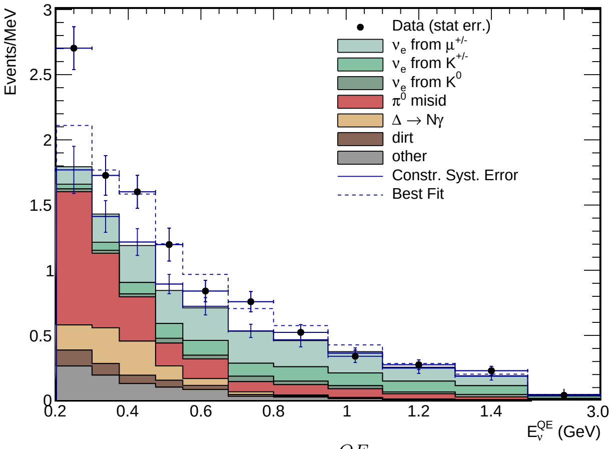


FIG. 15: The neutrino mode $E_\nu^{QE}$ distributions, corresponding to the second $6.38 \times 10^{20}$ POT data set, for $\nu_e$ CCQE data (points with statistical errors) and background (histogram with systematic errors).

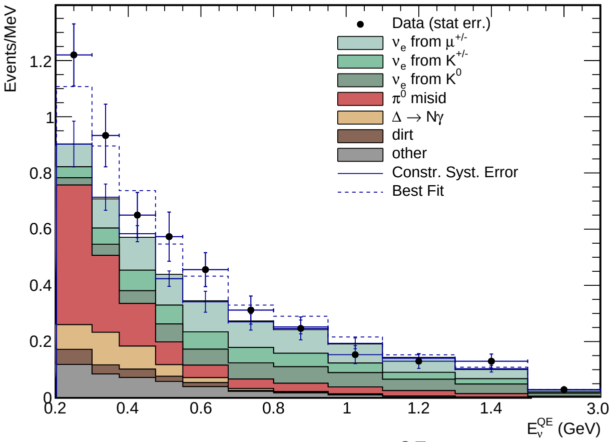


FIG. 16: The antineutrino mode $E_\nu^{QE}$ distributions, corresponding to the published $11.27 \times 10^{20}$ POT data, for $\nu_e$ CCQE data (points with statistical errors) and background (histogram with systematic errors).
